# Supplementary material for: Evaluating Self-Supervised Learning for Molecular Graph Embeddings
Source: arXiv:2206.08005 source file (2023-10-18)
Supplement: Supplementary file 1 [file structural_metric_appendix.tex]

\begin{table}[H]
\caption{Performance on the topological metrics predictions. We report the mean square or the cross entropy loss (\ie the smaller the better), over all 8 downstream datasets. 
We vary the amount of pre-training data (\ie GEOM) from 5k/10k/50k/100k/200k/330k(all) molecules.
We use ``$\uparrow$'' to represent the performance increases as the data quantity increases, ``$\downarrow$'' to represent the increase of the pre-train data hurdle the performance, ``$-$'' to represent there is no rules observed.
\label{tab:probe_appendix}}
\vspace{2ex}
% \small
\setlength{\tabcolsep}{4pt}
\centering
\begin{tabular}{l | c c c | c c c | c c c c}
\toprule
Metrics & \multicolumn{3}{c|}{Node} & \multicolumn{3}{c|}{Pair} & \multicolumn{4}{c}{Graph}\\
\midrule
Pre-training & Degree & Cent. & Cluster & Link & Jaccord & Katz & Diameter & Con. & Cycle & Assort. \\
\midrule
\method{AttrMask}     & $\uparrow$ & - & $\uparrow$ &  - & $\downarrow$ & $\uparrow$ & - & $\downarrow$ & - & $\downarrow$ \\
\method{GPT-GNN}      & $\uparrow$ & - & $\uparrow$ &  -& - & $\uparrow$ & - & $\uparrow$ & - & $\downarrow$ \\
\method{InfoGraph}    & $\downarrow$ & - & $\uparrow$ &  - & $\downarrow$ & $\uparrow$ & - & - & - & - \\
\method{Cont.Pred}  & $\uparrow$ & $\uparrow$ & - & $\downarrow$ & -  & $\uparrow$ & - & $\uparrow$ & - & $\downarrow$ \\
\method{G-Motif}      & $\uparrow$ & - & $\uparrow$ &  -& $\downarrow$ & $\uparrow$ & - & - & - & $\downarrow$ \\
\method{G-Cont.} & $\uparrow$ & - & - &  - & $\downarrow$ & $\uparrow$ & $\uparrow$ & - &  - & - \\
\method{GraphCL}      & - & - & $\uparrow$ & $\downarrow$ & - & $\uparrow$ &  $\uparrow$ & - & $\downarrow$ & $\uparrow$ \\
\method{JOAO}         & $\uparrow$ & - & $\downarrow$ &  - & $\downarrow$ & $\uparrow$ & - & $\uparrow$ & - & $\downarrow$ \\
\method{JOAOv2}       & $\uparrow$ & - & $\downarrow$ &  - & $\downarrow$ & $\uparrow$ & - & $\downarrow$ & - & $\downarrow$ \\
\midrule
\bottomrule
\end{tabular}
\end{table}
